# Supplementary material for: Safe Control Synthesis for Hybrid Systems through Local Control Barrier Functions
Source: arXiv:2311.17201 source file (2023-11-28)
Supplement: Supplementary file 1 [file appendix.tex]

\section*{Appendix}\label{sec:appendix}

\def\ourtextwidth{0.15}

\begin{figure}[!h]
  \centering
    \begin{subfigure}[b]{\ourtextwidth\textwidth}
    \includegraphics[width=\textwidth]{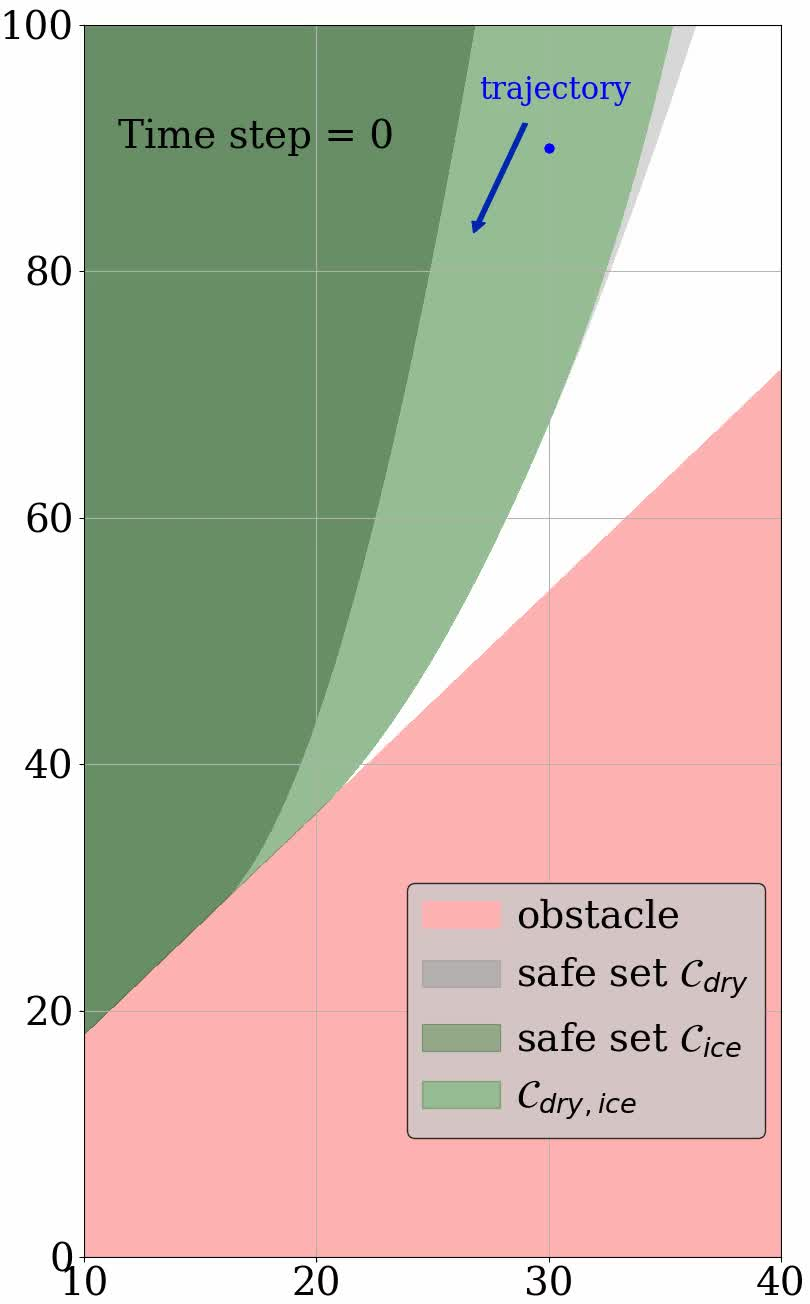}
    \label{fig:ours-good-01}
  \end{subfigure}
  \begin{subfigure}[b]{\ourtextwidth\textwidth}
    \includegraphics[width=\textwidth]{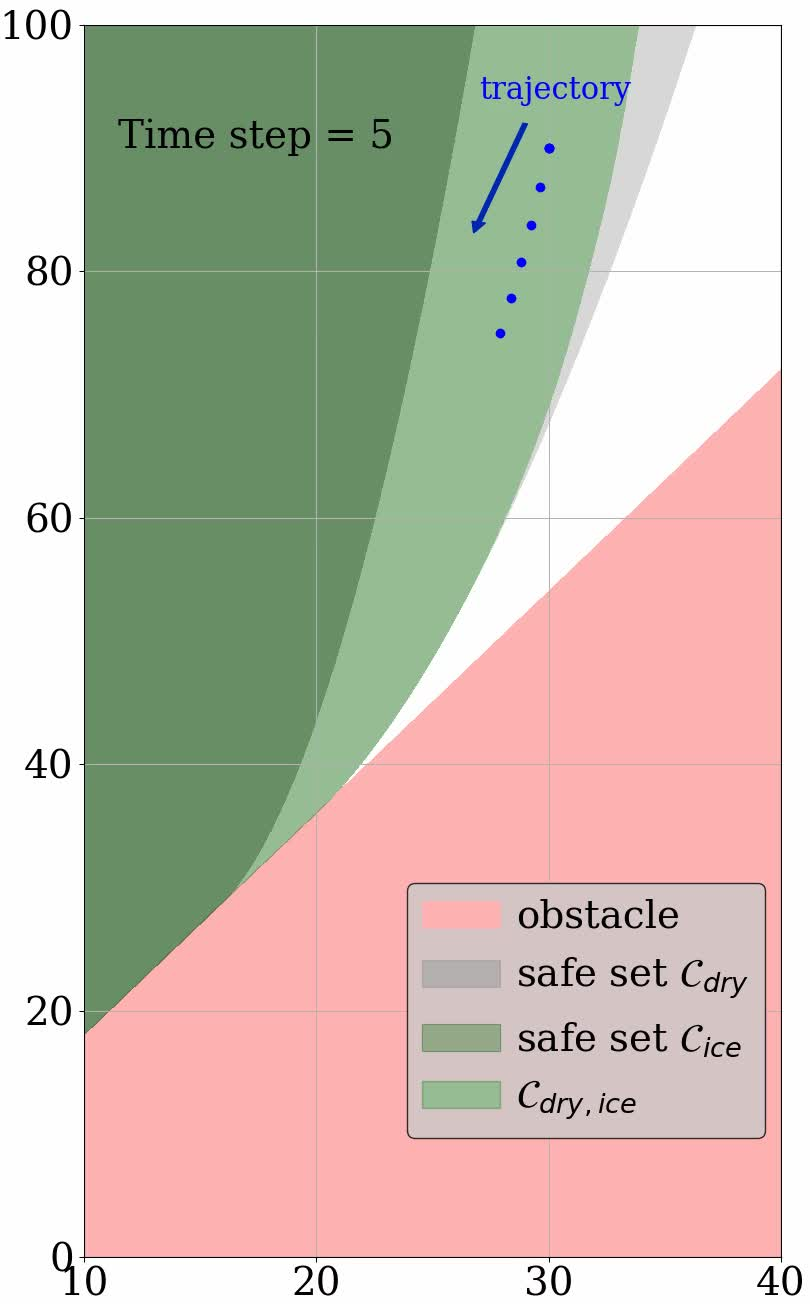}
    \label{fig:ours-good-06}
  \end{subfigure}
    \begin{subfigure}[b]{\ourtextwidth\textwidth}
    \includegraphics[width=\textwidth]{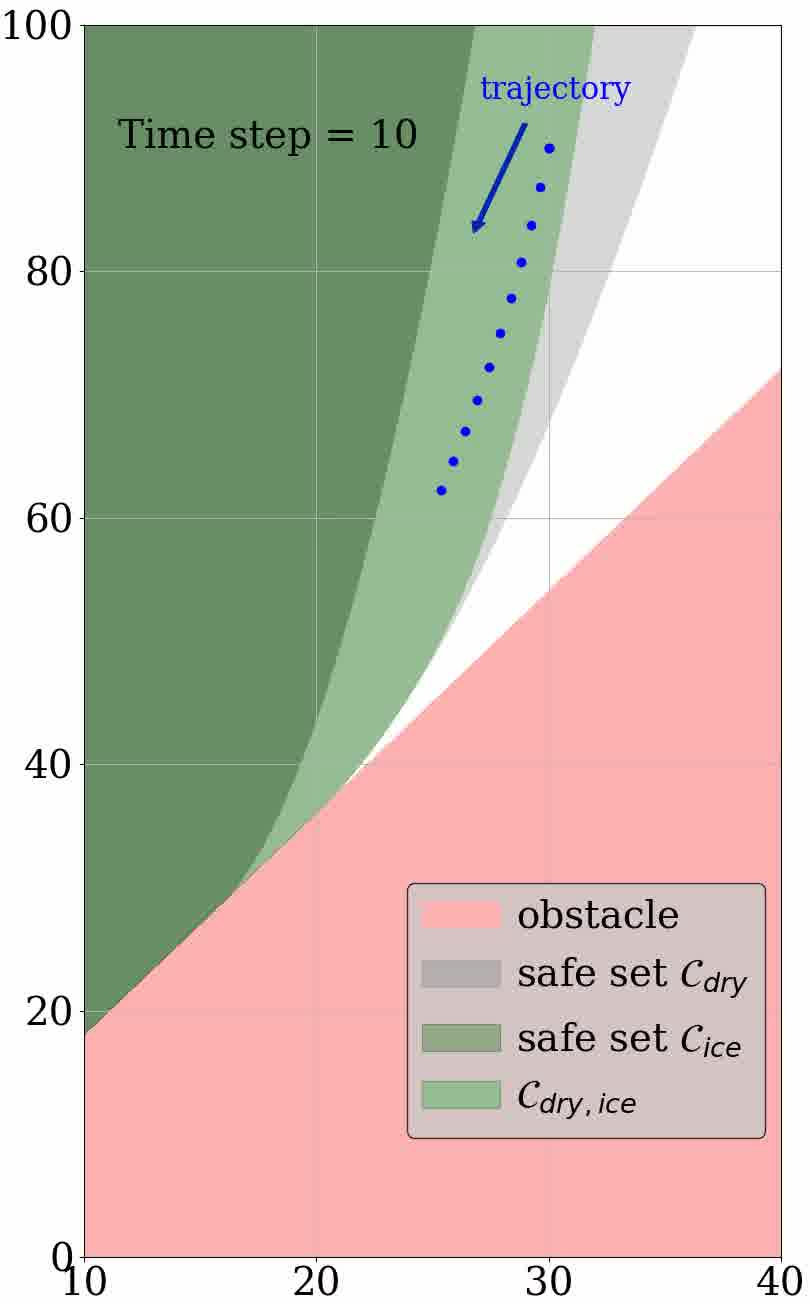}
    \label{fig:ours-good-11}
  \end{subfigure}
    \begin{subfigure}[b]{\ourtextwidth\textwidth}
    \includegraphics[width=\textwidth]{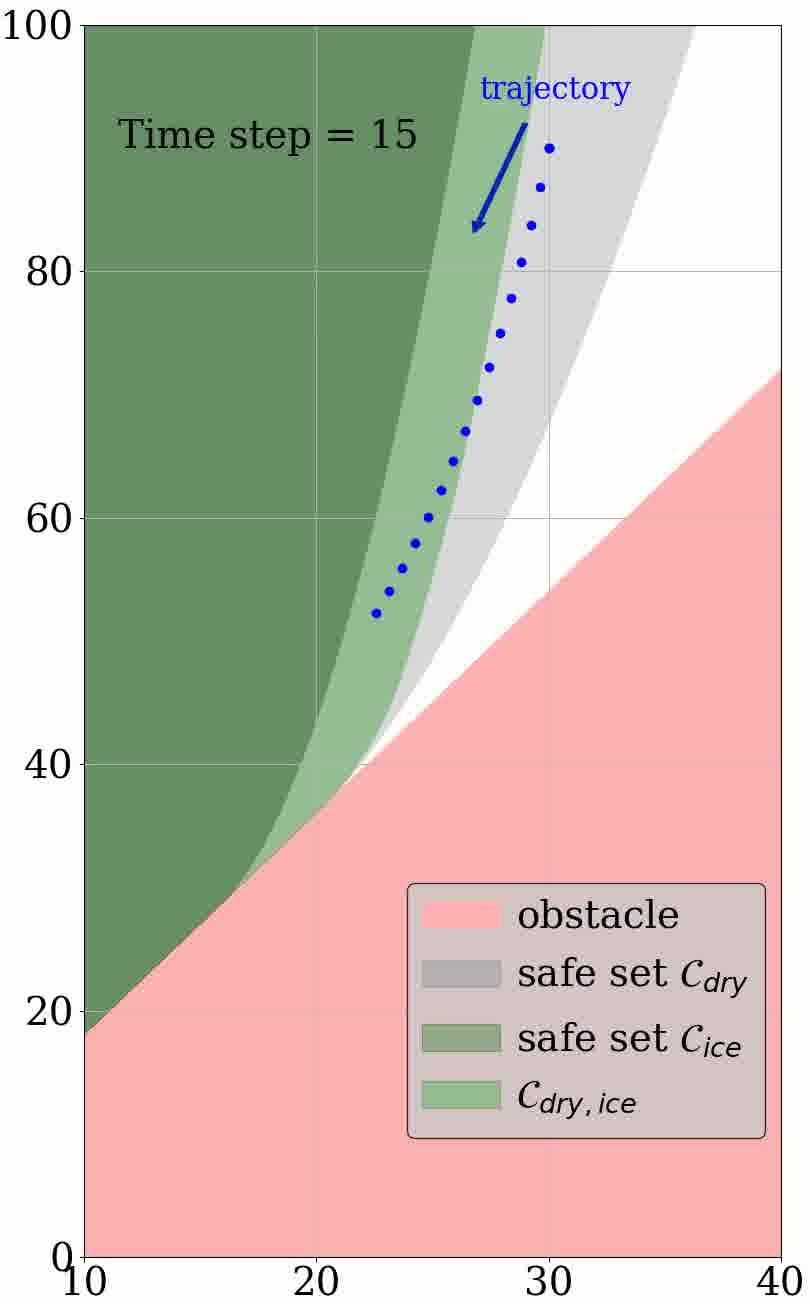}
    \label{fig:ours-good-16}
  \end{subfigure}
      \begin{subfigure}[b]{\ourtextwidth\textwidth}
    \includegraphics[width=\textwidth]{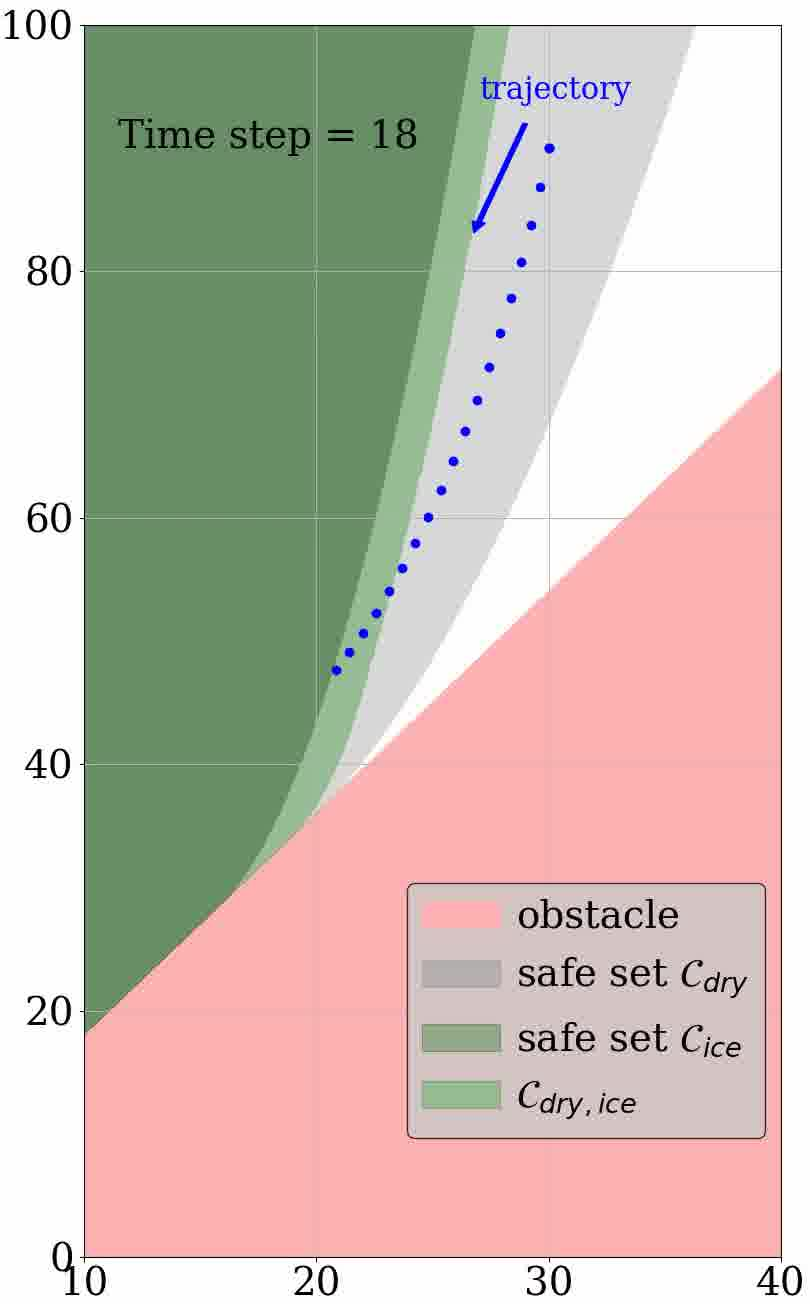}
    \label{fig:ours-good-19}
  \end{subfigure}
      \begin{subfigure}[b]{\ourtextwidth\textwidth}
    \includegraphics[width=\textwidth]{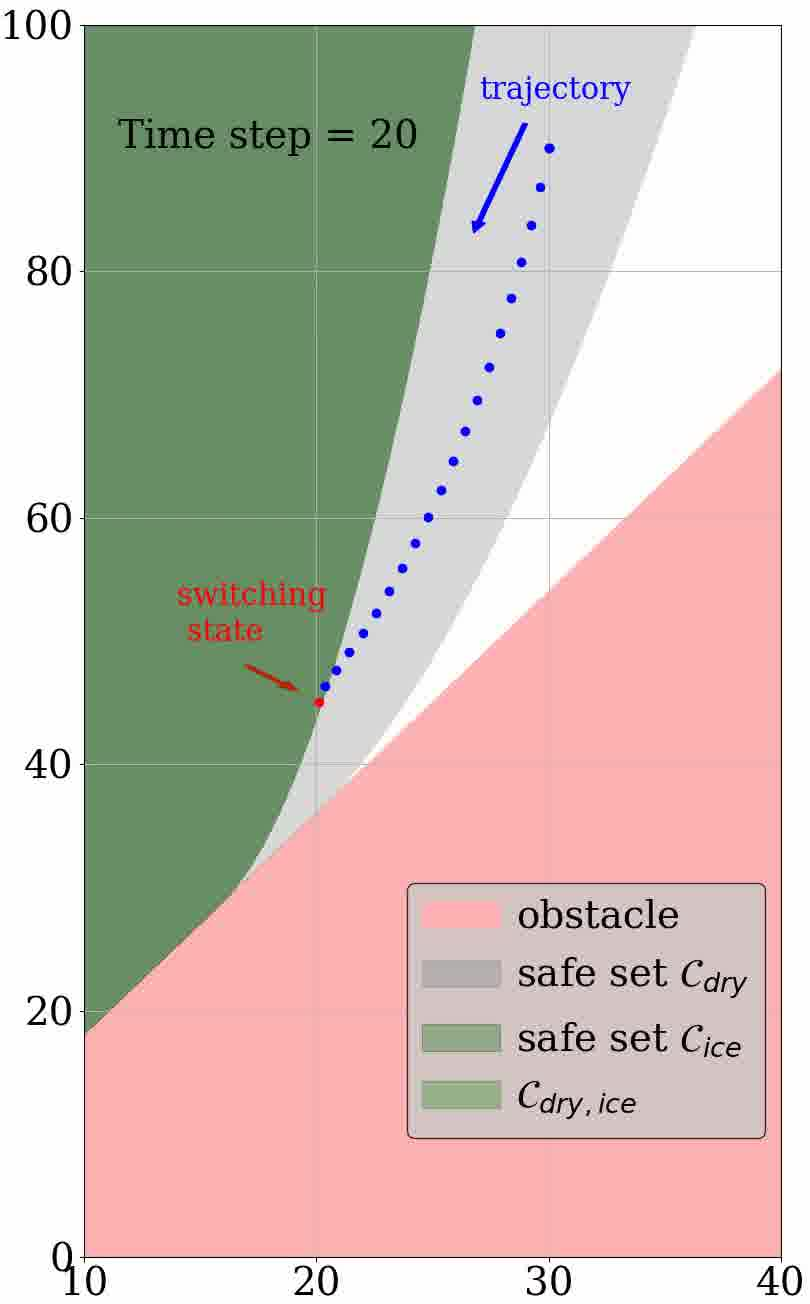}
    \label{fig:ours-good-21}
  \end{subfigure}
        \begin{subfigure}[b]{\ourtextwidth\textwidth}
    \includegraphics[width=\textwidth]{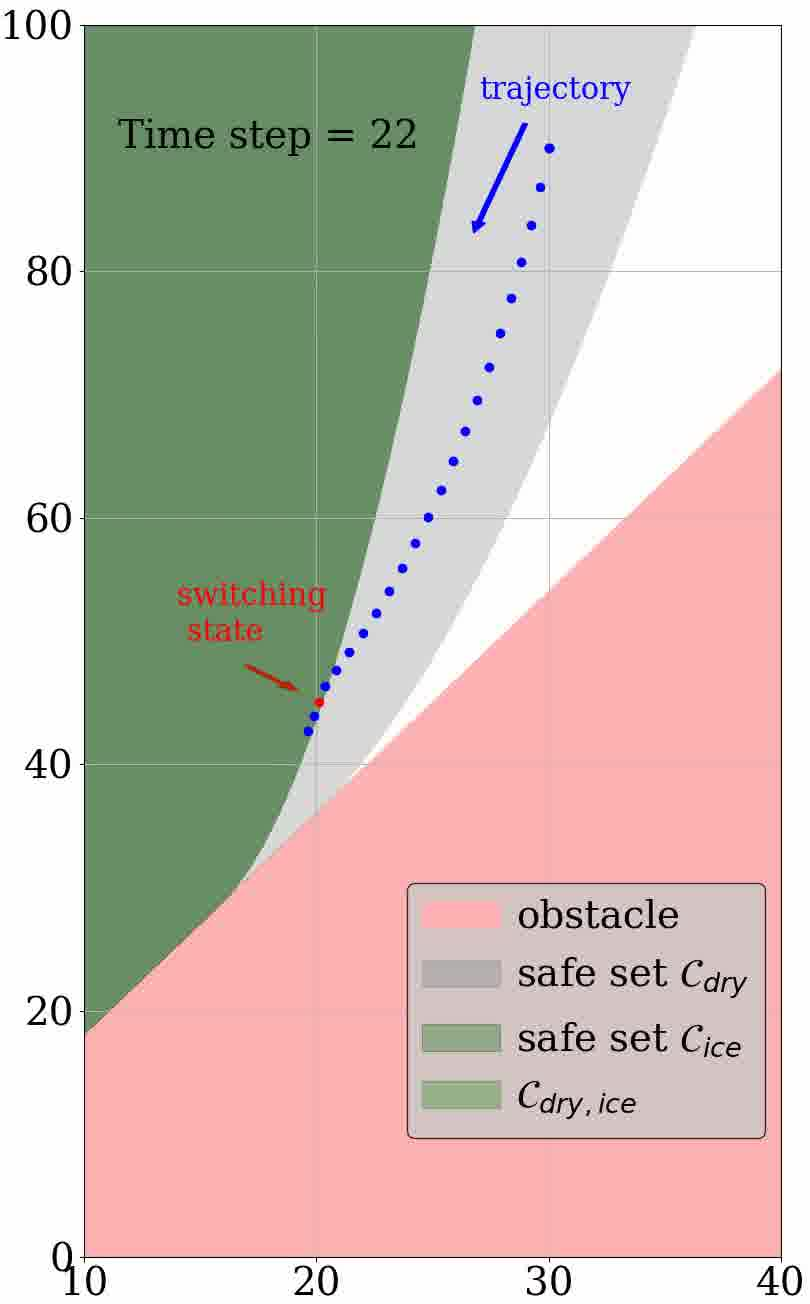}
    \label{fig:ours-good-23}
  \end{subfigure}
      \begin{subfigure}[b]{\ourtextwidth\textwidth}
    \includegraphics[width=\textwidth]{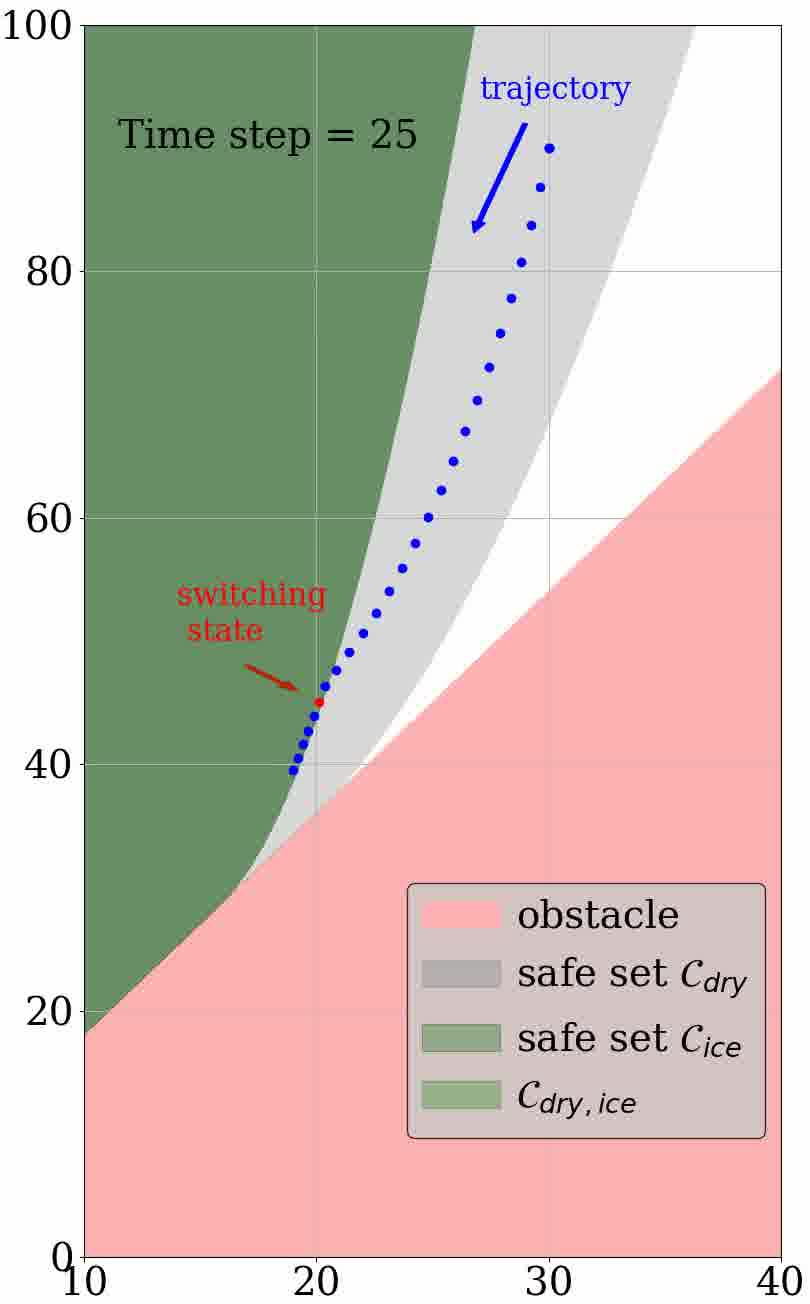}
    \label{fig:ours-good-26}
  \end{subfigure}
        \begin{subfigure}[b]{\ourtextwidth\textwidth}
    \includegraphics[width=\textwidth]{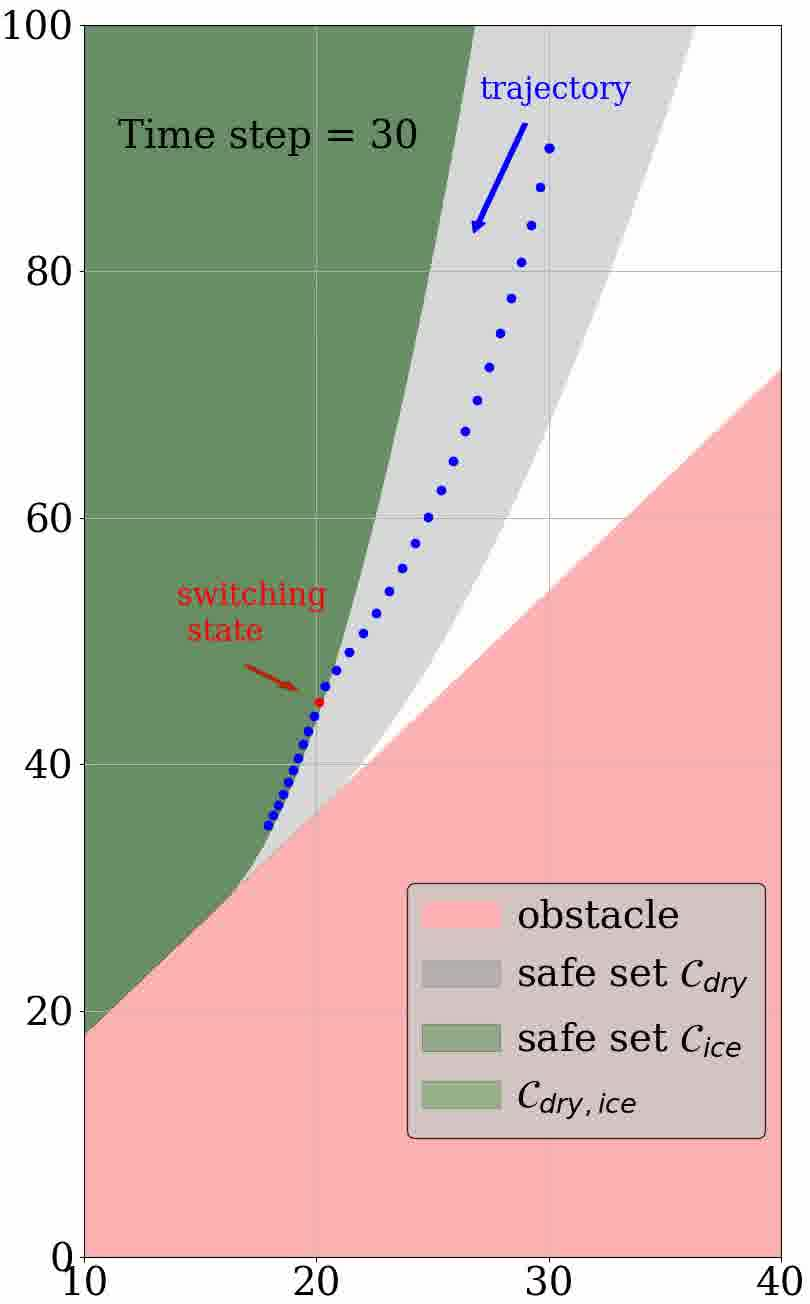}
    \label{fig:ours-good-31}
  \end{subfigure}
      \begin{subfigure}[b]{\ourtextwidth\textwidth}
    \includegraphics[width=\textwidth]{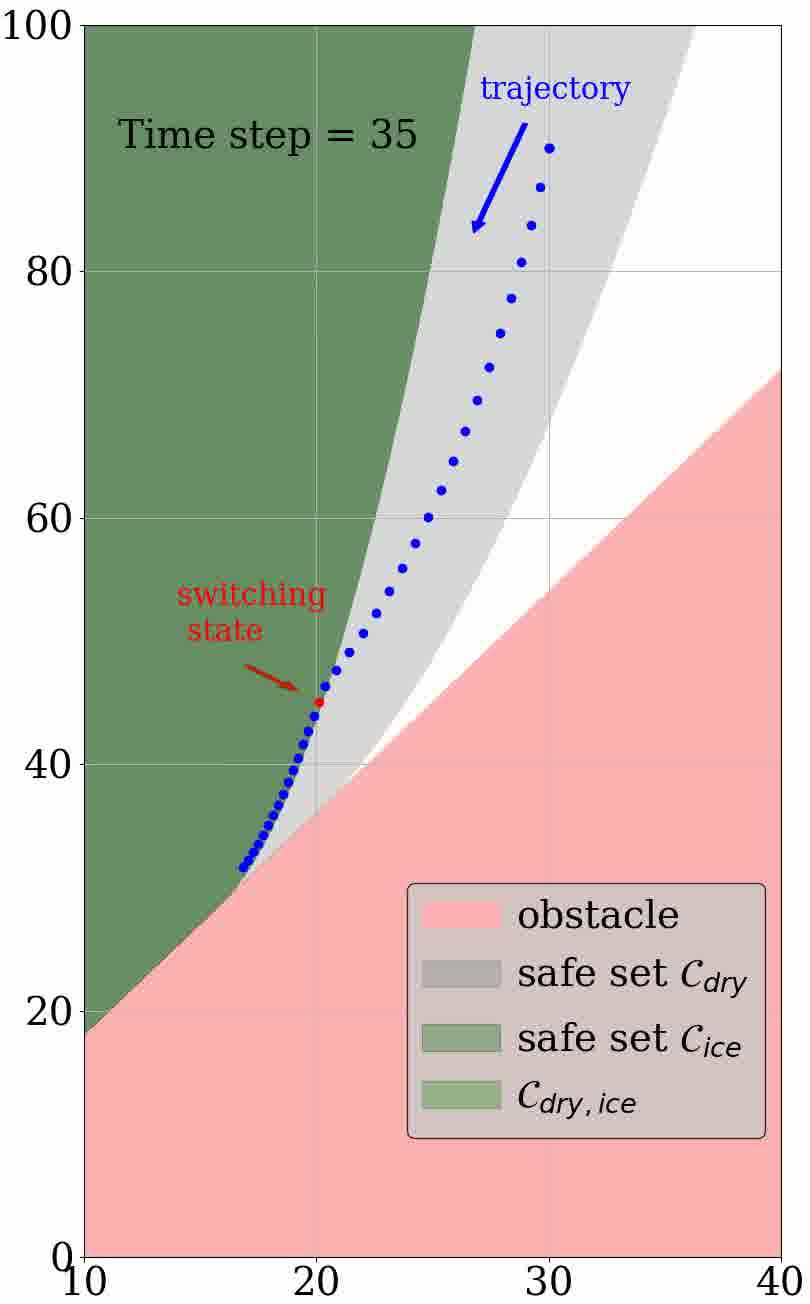}
    \label{fig:ours-good-36}
  \end{subfigure}
        \begin{subfigure}[b]{\ourtextwidth\textwidth}
    \includegraphics[width=\textwidth]{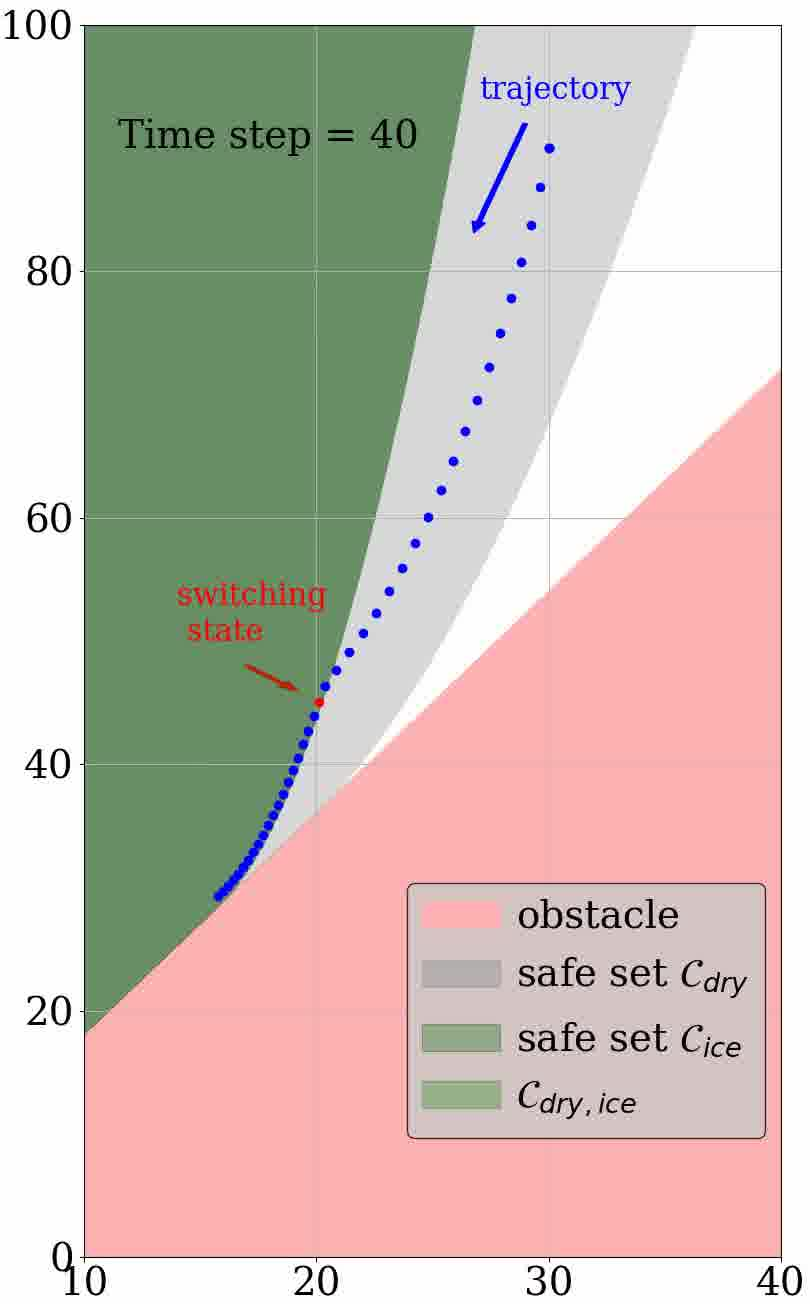}
    \label{fig:ours-good-41}
  \end{subfigure}
      \begin{subfigure}[b]{\ourtextwidth\textwidth}
    \includegraphics[width=\textwidth]{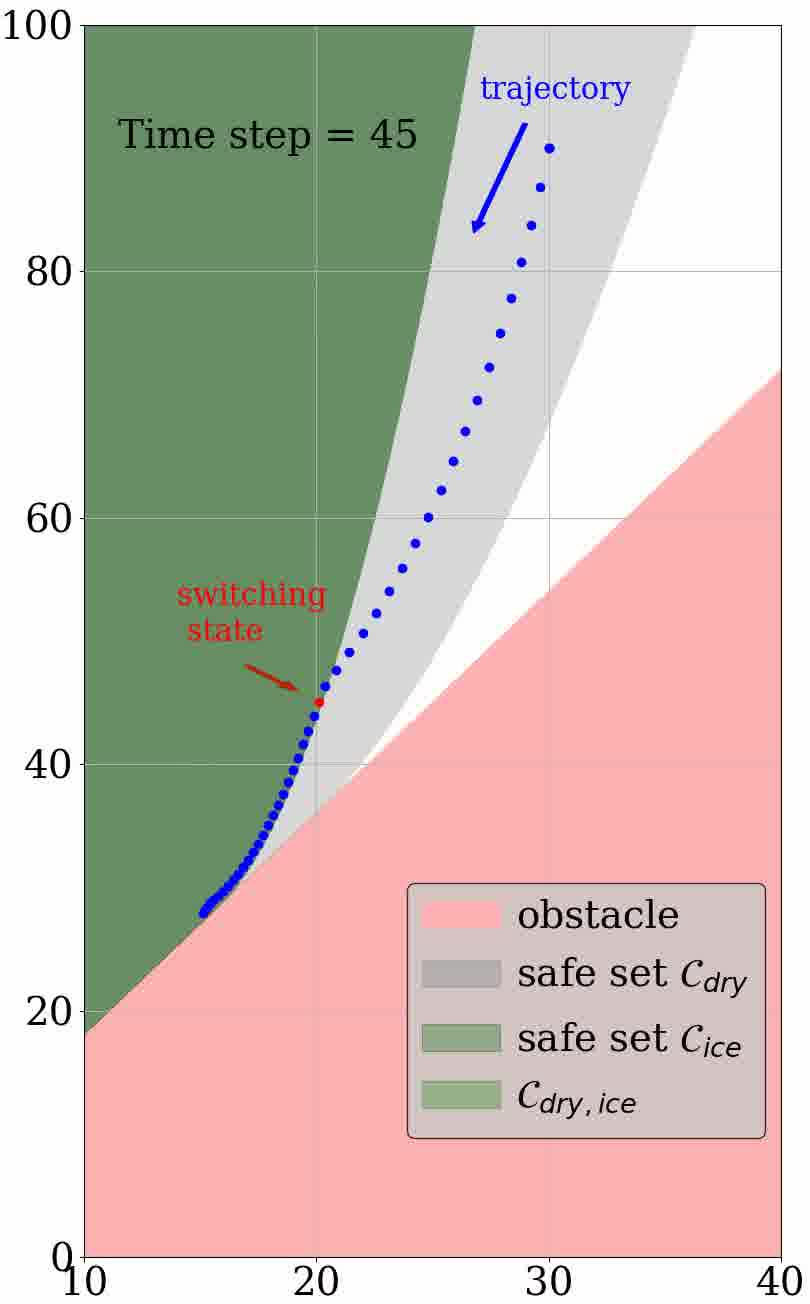}
    \label{fig:ours-good-46}
  \end{subfigure}
  \caption{Snapshots for the trajectory with our approach.}
\end{figure}

\begin{figure}[!h]
  \centering
    \begin{subfigure}[b]{\ourtextwidth\textwidth}
    \includegraphics[width=\textwidth]{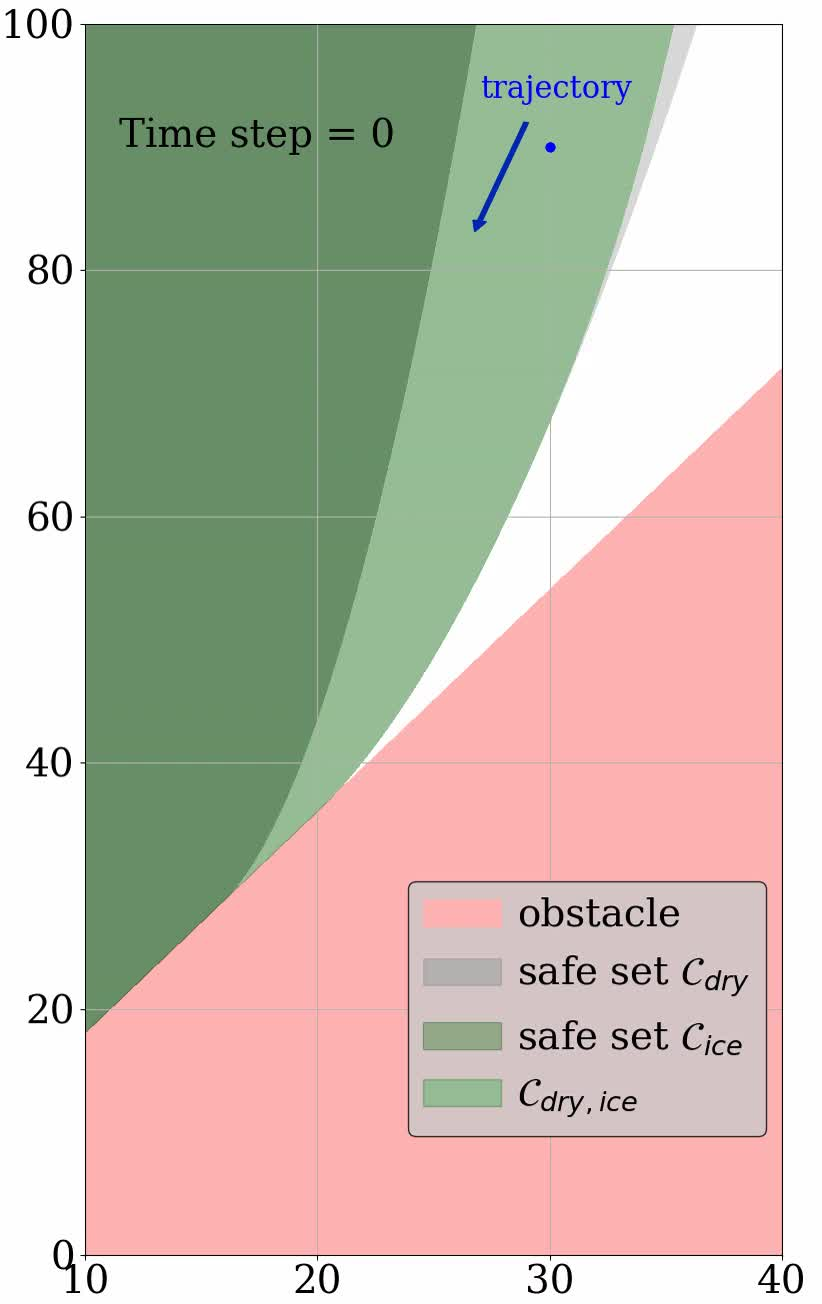}
    \label{fig:ours-bad-01}
  \end{subfigure}
  \begin{subfigure}[b]{\ourtextwidth\textwidth}
    \includegraphics[width=\textwidth]{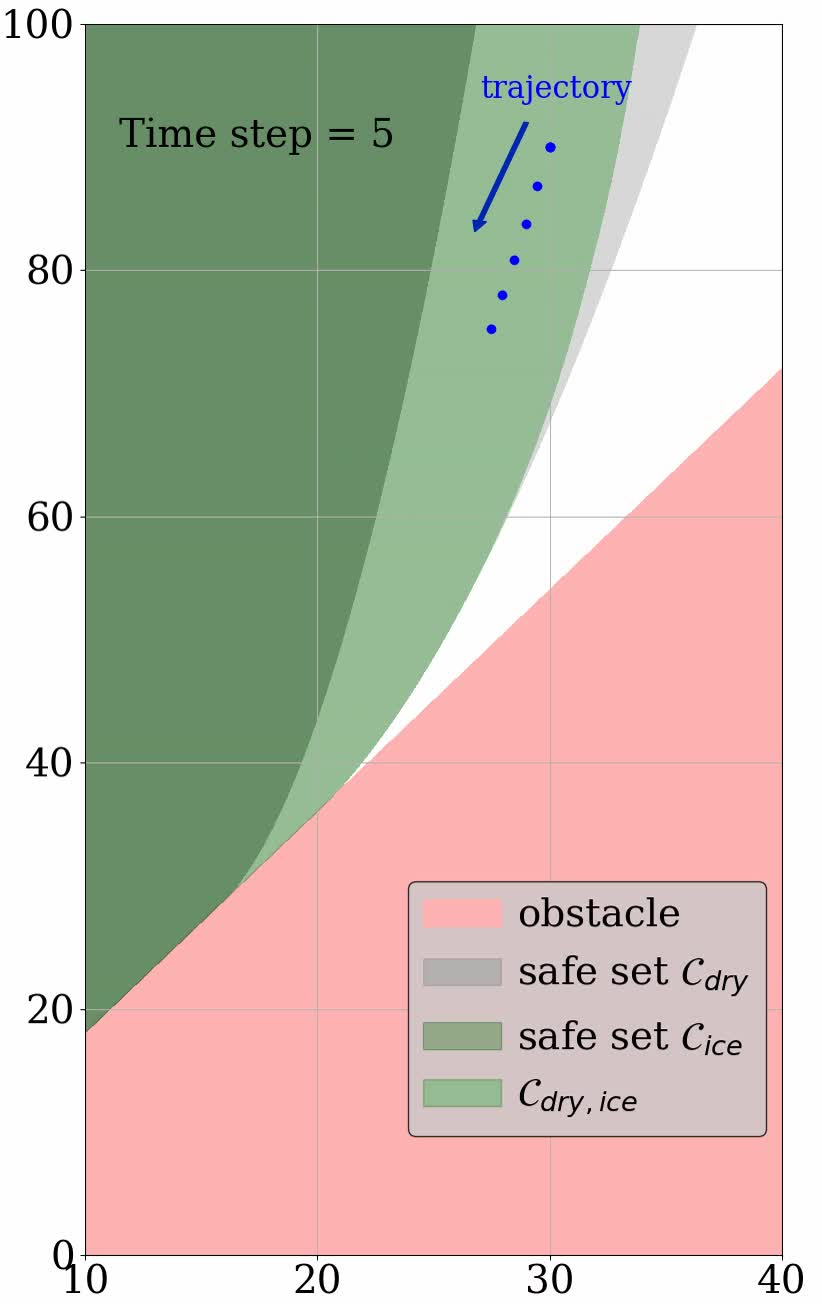}
    \label{fig:ours-bad-06}
  \end{subfigure}
    \begin{subfigure}[b]{\ourtextwidth\textwidth}
    \includegraphics[width=\textwidth]{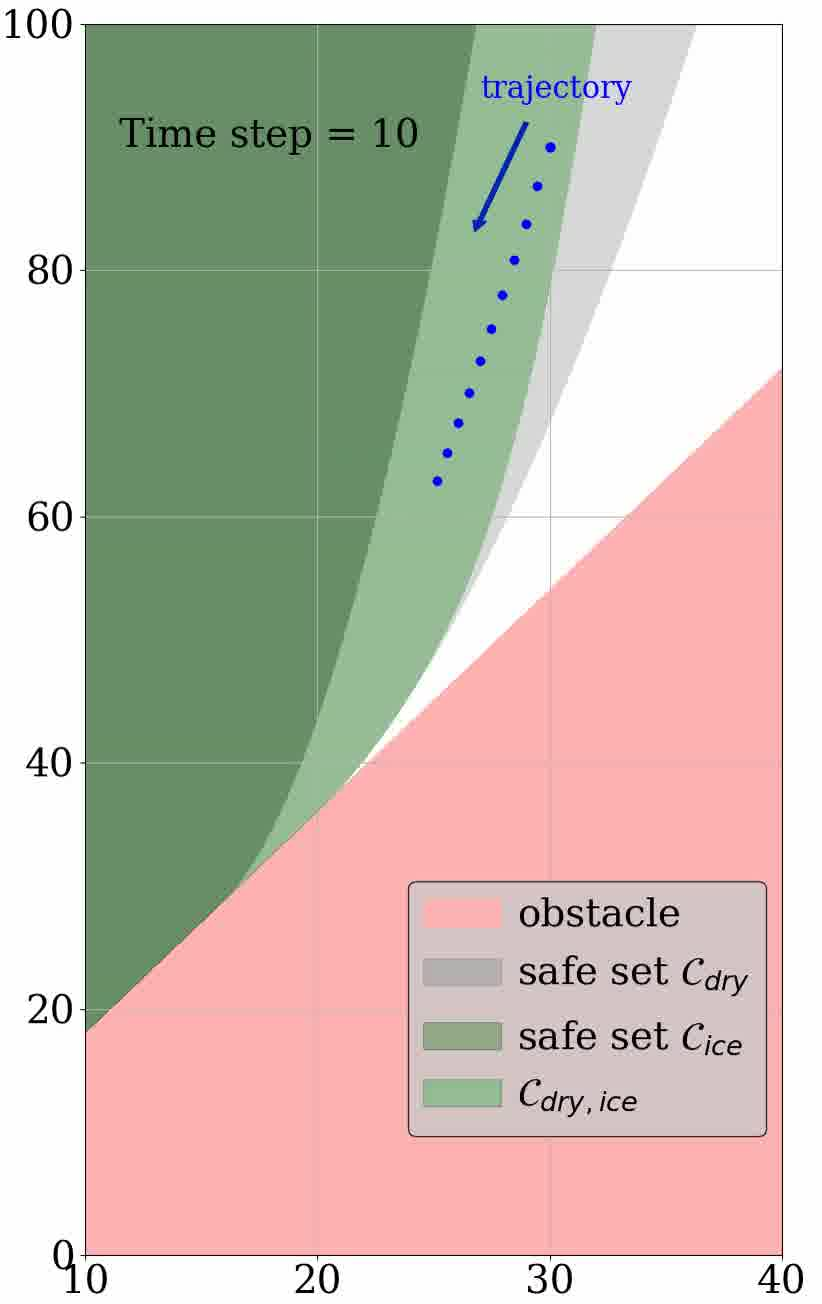}
    \label{fig:ours-bad-11}
  \end{subfigure}
    \begin{subfigure}[b]{\ourtextwidth\textwidth}
    \includegraphics[width=\textwidth]{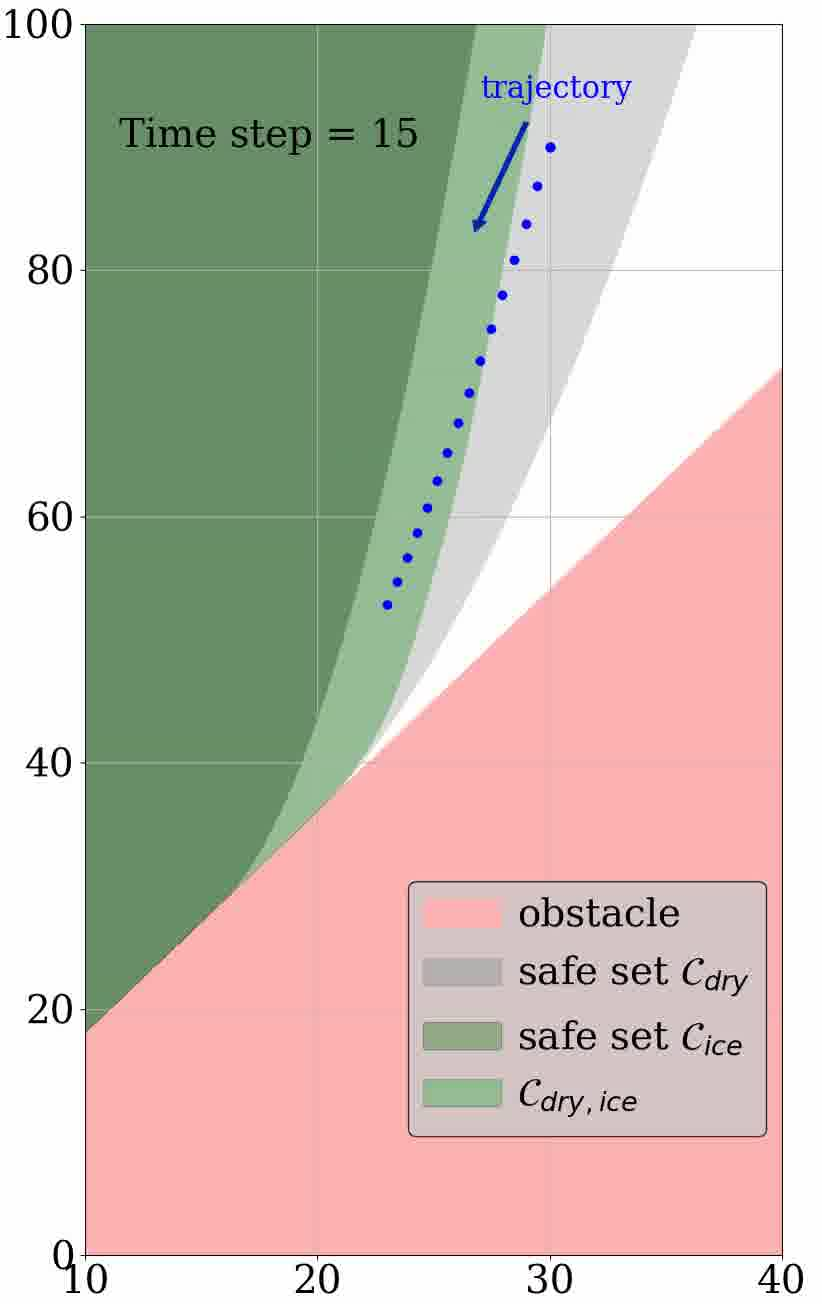}
    \label{fig:ours-bad-16}
  \end{subfigure}
      \begin{subfigure}[b]{\ourtextwidth\textwidth}
    \includegraphics[width=\textwidth]{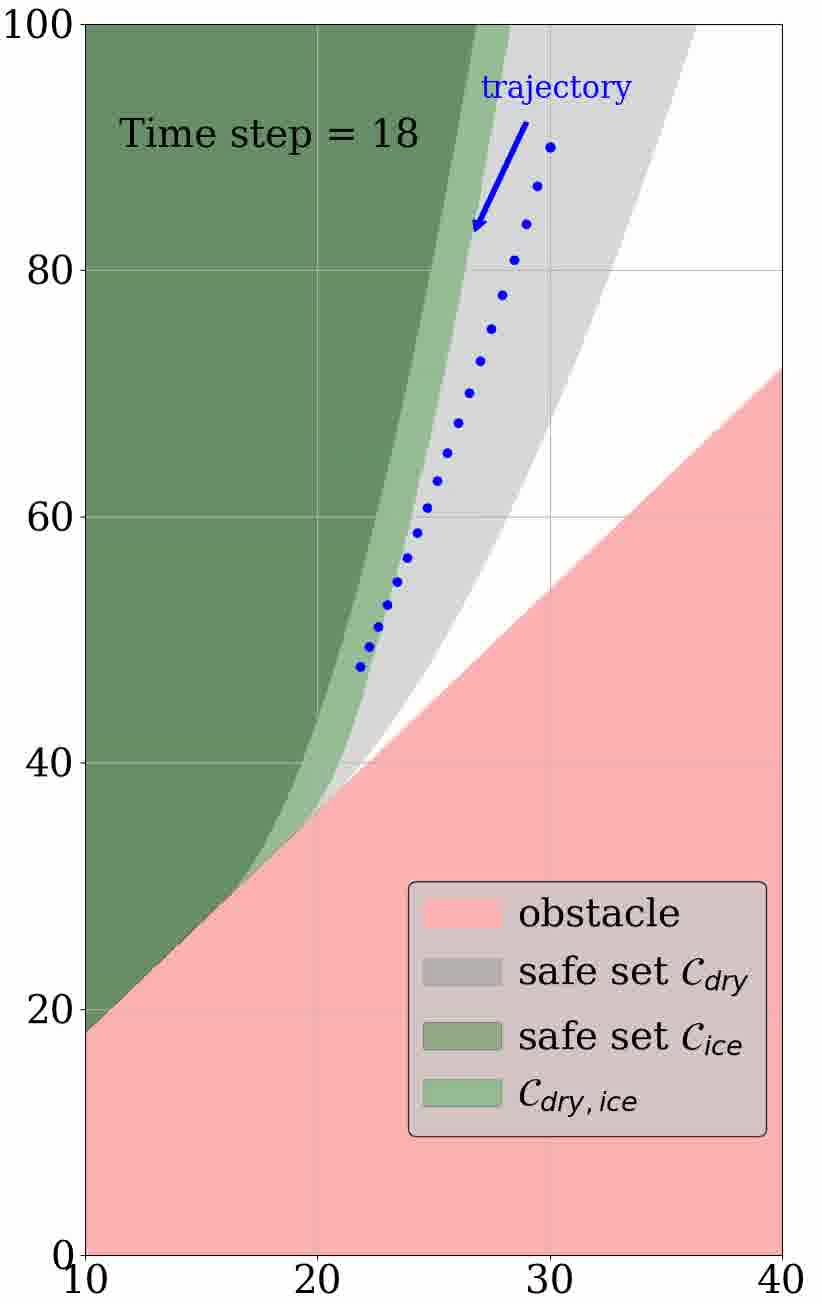}
    \label{fig:ours-bad-19}
  \end{subfigure}
      \begin{subfigure}[b]{\ourtextwidth\textwidth}
    \includegraphics[width=\textwidth]{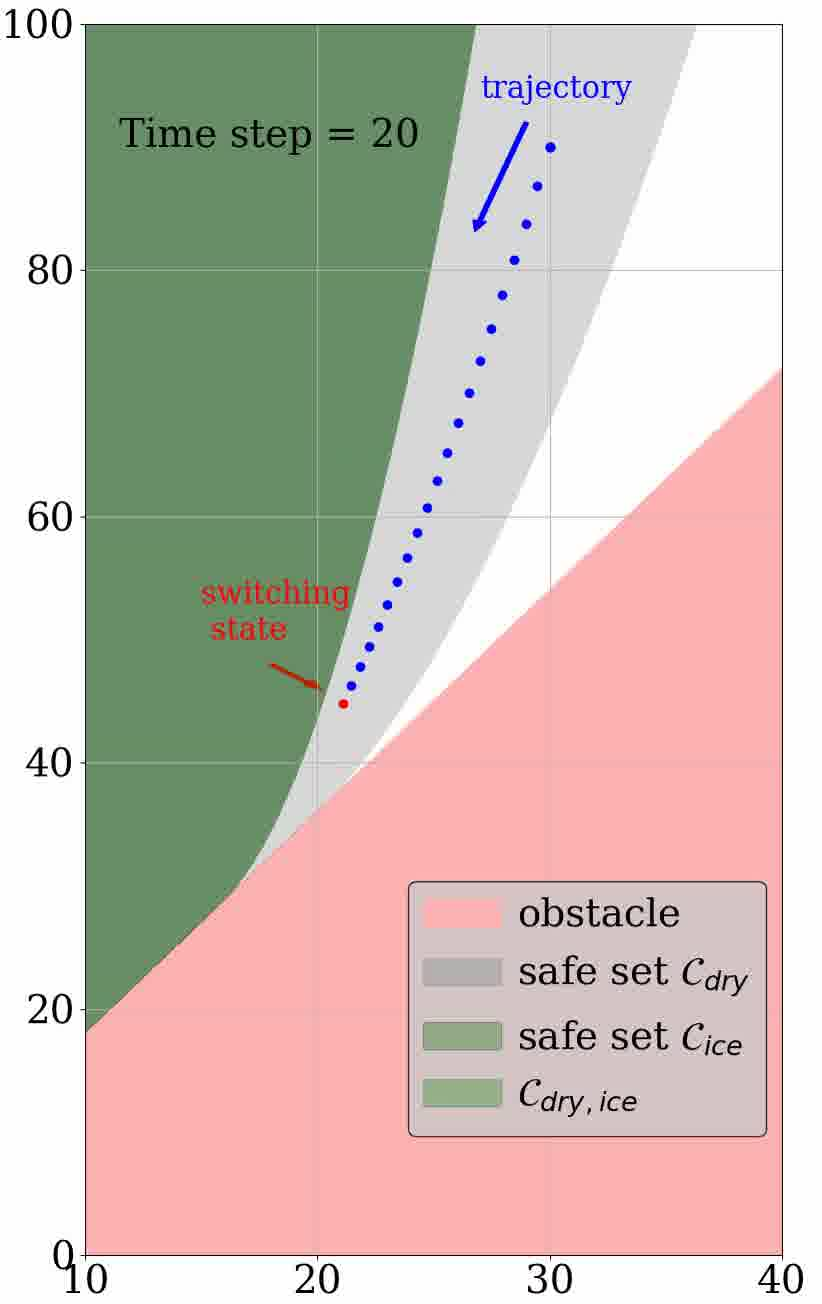}
    \label{fig:ours-bad-21}
  \end{subfigure}
        \begin{subfigure}[b]{\ourtextwidth\textwidth}
    \includegraphics[width=\textwidth]{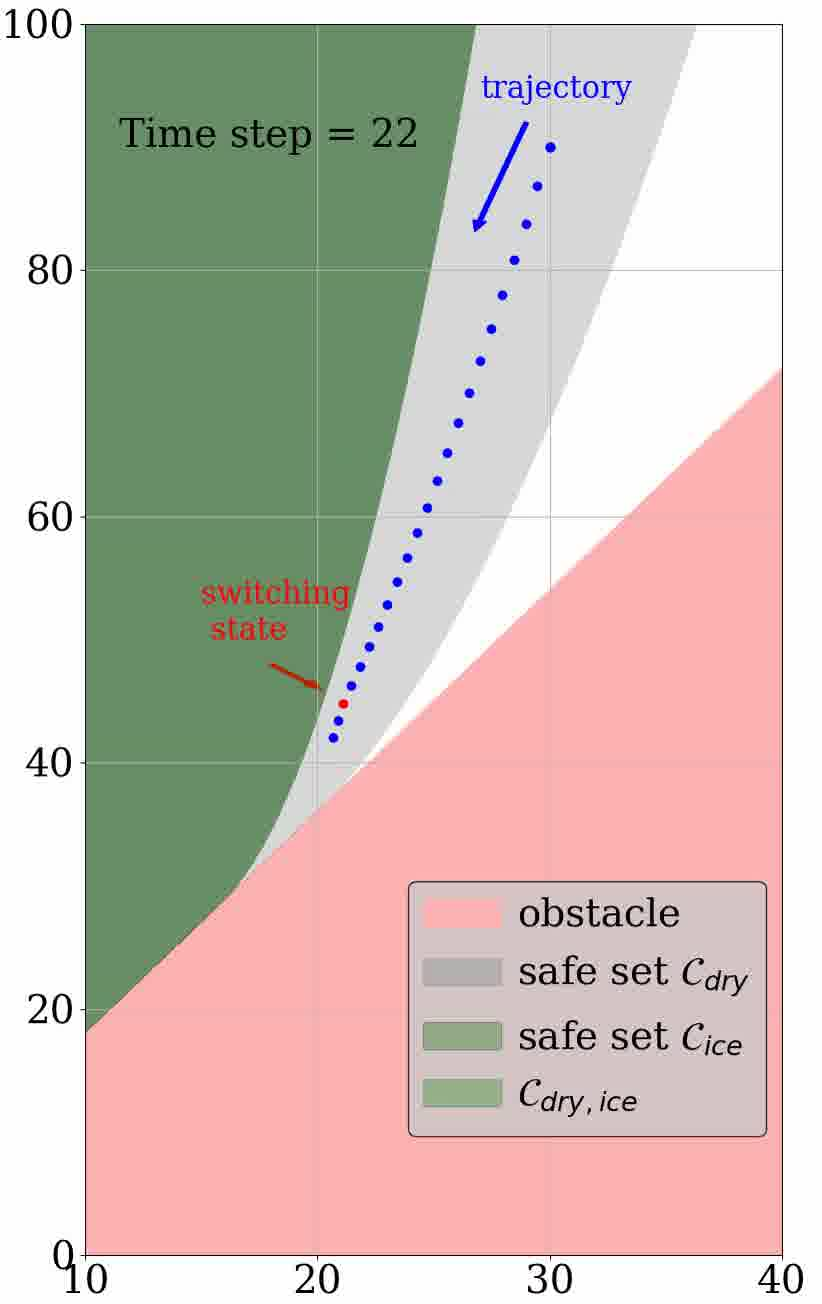}
    \label{fig:ours-bad-23}
  \end{subfigure}
      \begin{subfigure}[b]{\ourtextwidth\textwidth}
    \includegraphics[width=\textwidth]{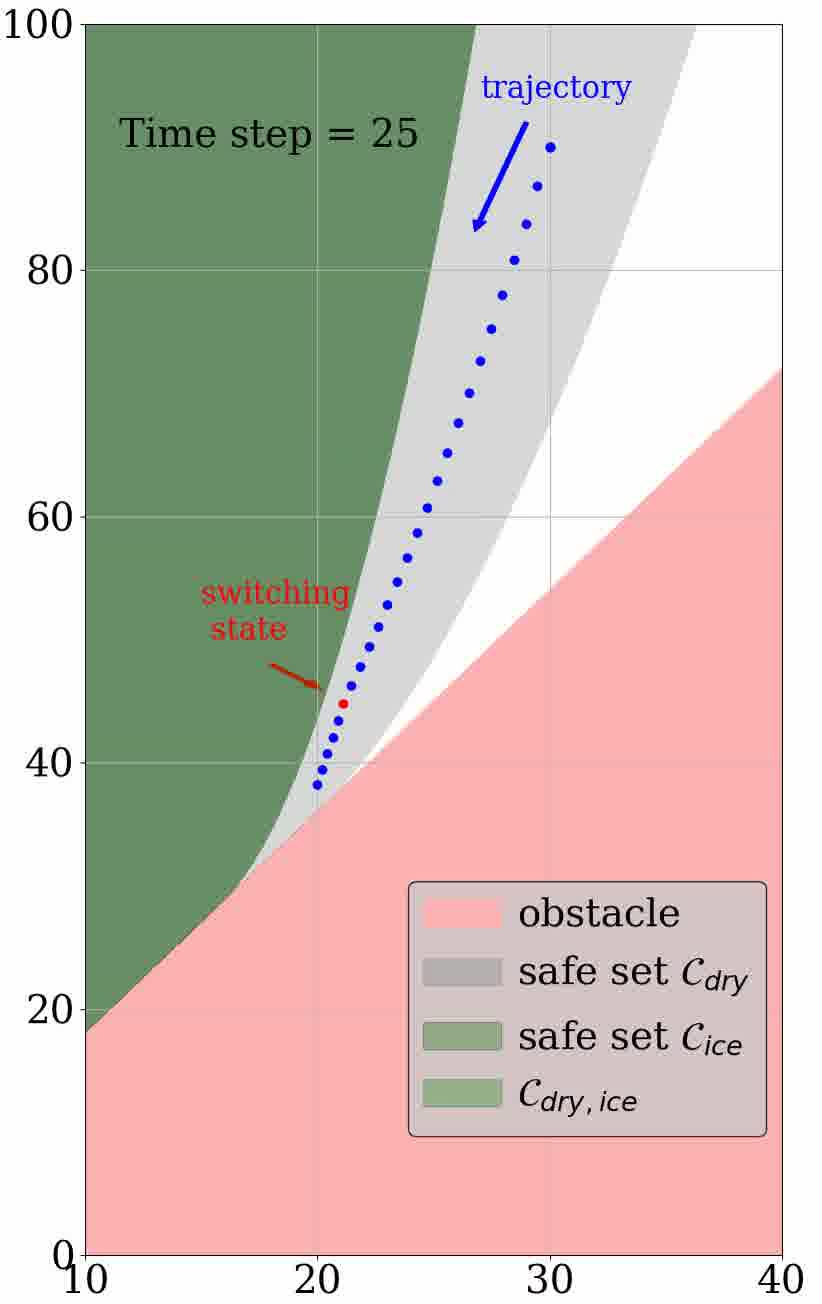}
    \label{fig:ours-bad-26}
  \end{subfigure}
        \begin{subfigure}[b]{\ourtextwidth\textwidth}
    \includegraphics[width=\textwidth]{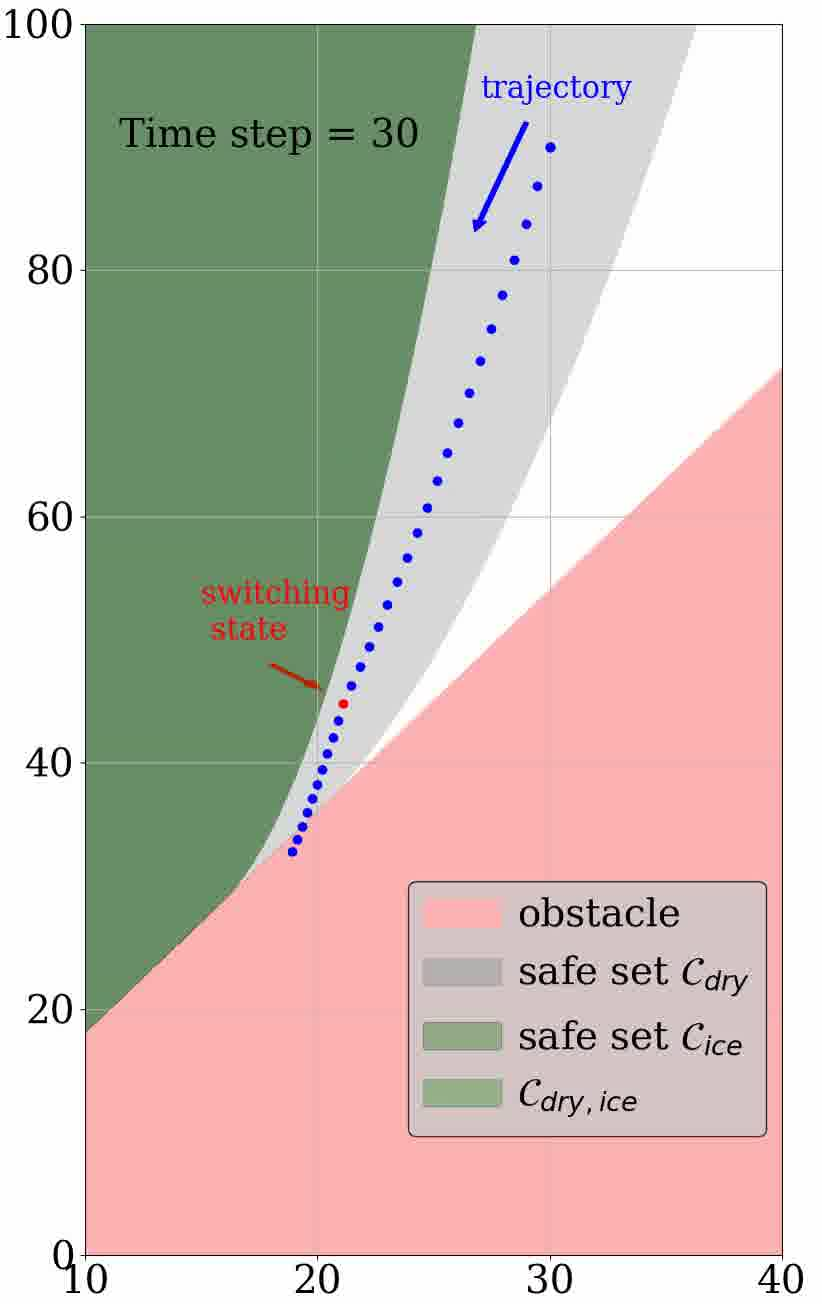}
    \label{fig:ours-bad-31}
  \end{subfigure}
      \begin{subfigure}[b]{\ourtextwidth\textwidth}
    \includegraphics[width=\textwidth]{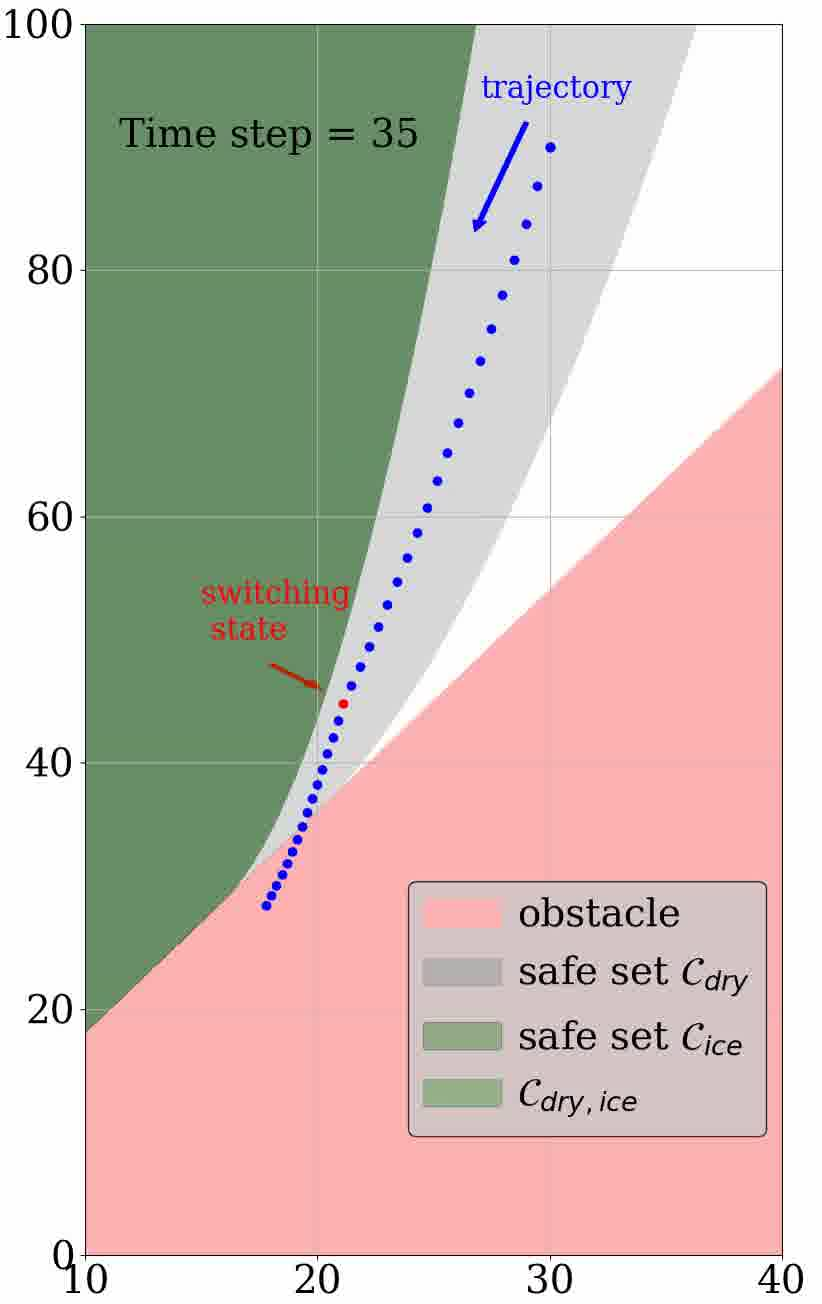}
    \label{fig:ours-bad-36}
  \end{subfigure}
        \begin{subfigure}[b]{\ourtextwidth\textwidth}
    \includegraphics[width=\textwidth]{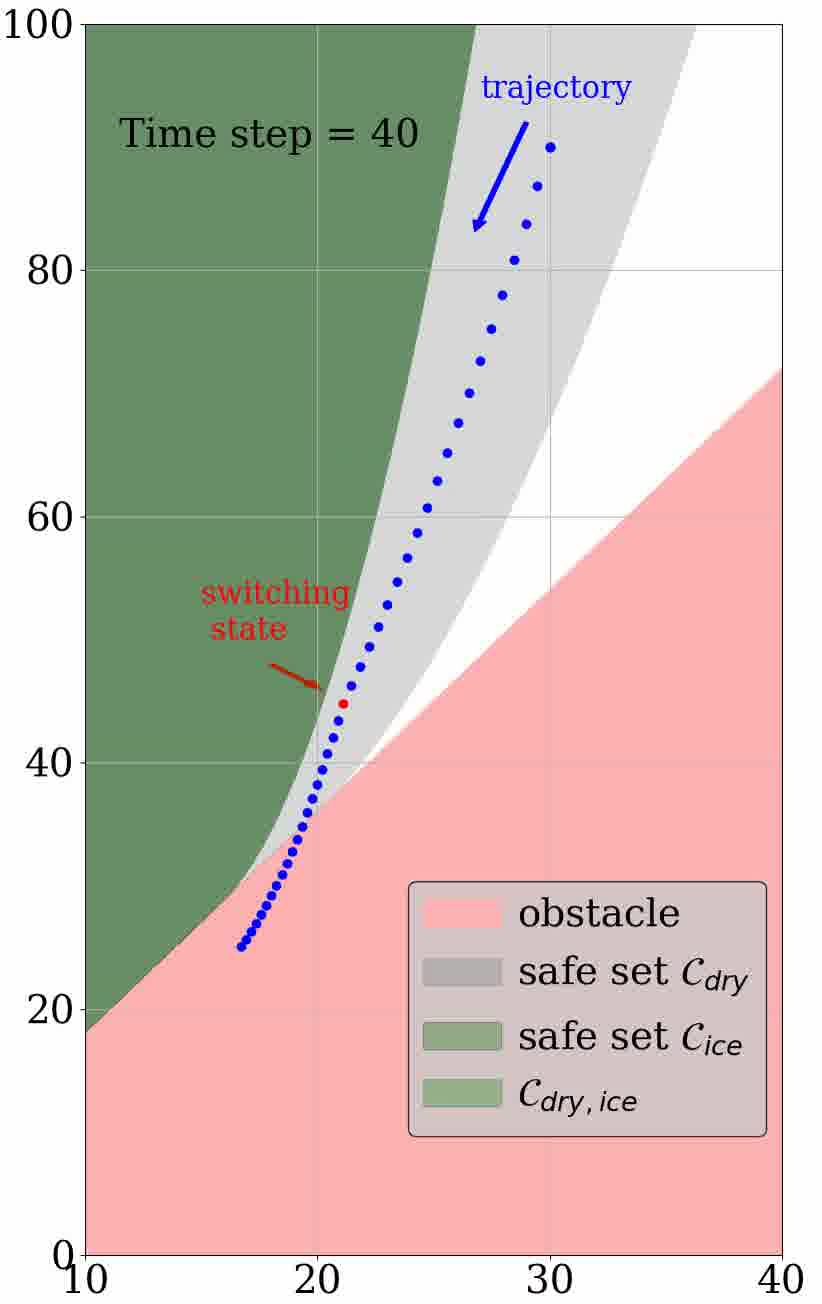}
    \label{fig:ours-bad-41}
  \end{subfigure}
      \begin{subfigure}[b]{\ourtextwidth\textwidth}
    \includegraphics[width=\textwidth]{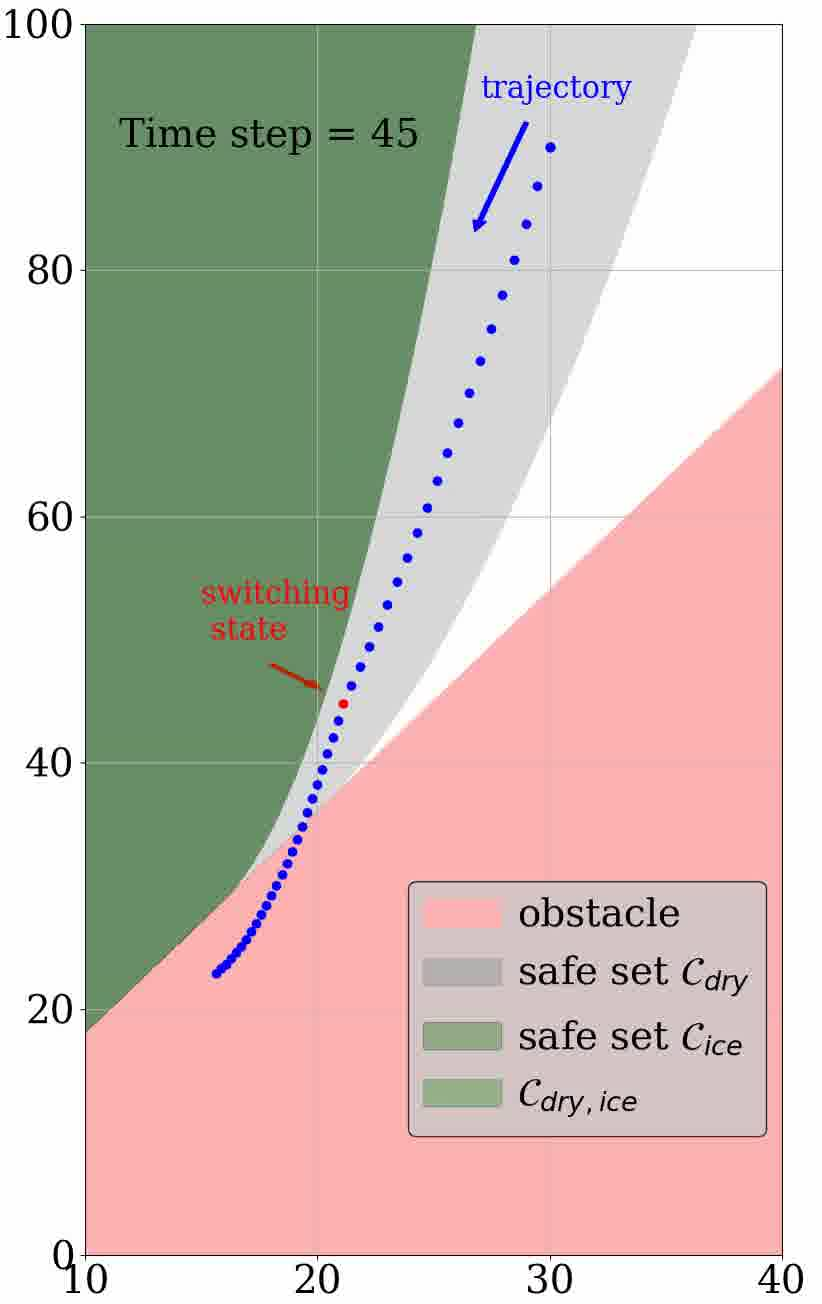}
    \label{fig:ours-bad-46}
  \end{subfigure}
  \caption{Snapshots for the trajectory with baseline approach.}
\end{figure}
